# Supplementary material for: Zeno-clocking the Auger decay
Source: arXiv:1804.06605 ancillary file (2018-12-11)
Supplement: Supplementary file 1 [file zeno_SM.pdf]

# Supplementary material to: Time-stretched spectroscopy by quantum Zeno effect: The case of the Auger decay

E. Viñas Boström,[1,2] M. Gisselbrecht,[1] T. Brage,[1] C.-O. Almbladh,[1,2] A. Mikkelsen,[1] and C. Verdozzi[1,2]

[1]*Lund University, Department of Physics, PO Box 118, 221 00 Lund, Sweden*
[2]*European Theoretical Spectroscopy Facility (ETSF)*

(Dated: September 10, 2018)

## I. HAMILTONIAN IN THE TWO-PARTICLE BASIS

In this section we show how the effective Hamiltonian used in the main text can be derived a many-body Hamiltonian written in terms of single-particle orbitals.

We consider a model atomic system, where a core electron has already been ejected and does not interact with the system left behind. This is the so-called sudden ejection limit[1], and is appropriate for high photo-electron energies, which can be achieved using high frequency radiation for the core ionization. The atom has two spinless electrons, which enter the Auger decay, and is exposed to a classical time-dependent light-field $E(t)$ treated in the dipole approximation. Our choice of a spinless model is computationally convenient, while fully retaining the qualitative aspects of Auger physics compared to the spinful case[2]. In an atomic orbital picture, the Hamiltonian characterising the system and radiation takes the form

$$H(t) = H_a + H_c + H_{int} + H_{ext}(t). \tag{1}$$

In Eq. (1), the atomic Hamiltonian $H_a$ is modeled in terms of four relevant atomic orbitals: $|c\rangle$, $|v_1\rangle$, $|v_2\rangle$ and $|v_3\rangle$. Here $|c\rangle$ is the core state (initially already empty), and $|v_1\rangle$ and $|v_2\rangle$ are initially occupied valence orbitals. These three states are taken with orbital $s$-symmetry. State $|v_3\rangle$, a valence state of higher energy, is of $p$-symmetry and initially empty. Thus, the atomic Hamiltonian is

$$\begin{aligned} H_a = \epsilon_c n_c + \sum_i \epsilon_{v_i} \hat{n}_{v_i} + \sum_i U_{ci} \hat{n}_c \hat{n}_{v_i} \\ + \sum_{i<j} U_{ij} \hat{n}_{v_i} \hat{n}_{v_j}, \end{aligned} \tag{2}$$

where $i, j \in (1, 2, 3)$, $\hat{n}_{v_i} = c^\dagger_{v_i} c_{v_i}$, and $c^\dagger_{v_i}$ creates a spinless electron in level $|v_i\rangle$ with orbital energy $\epsilon_{v_i}$. Similarly $\hat{n}_c = c^\dagger_c c_c$, where $c^\dagger_c$ creates a spinless electron in level $|c\rangle$ with energy $\epsilon_c$, and $U_{ij}$ is the strength of the intra-atomic Coulomb interactions.

In our description both the initial state $|\Psi_0\rangle = |v_1 v_2\rangle$ as well as the excited state $|v_1 v_3\rangle$ can undergo Auger decay. The term $H_c$ of Eq. (1) describes the Auger continuum states $|\epsilon_k\rangle$, grouped in two regions $\mathcal{S}$ and $\mathcal{P}$, respectively corresponding to states with $s$- and $p$-symmetry. According to the Auger selection rules, $\mathcal{S}$ ($\mathcal{P}$) provides the emission channel for the decay from state $|v_1 v_2\rangle$ ($|v_1 v_3\rangle$). Thus,

$$H_c = \sum_{k\in\mathcal{S}} \epsilon_k \hat{n}_k + \sum_{k\in\mathcal{P}} \epsilon_k \hat{n}_k. \tag{3}$$

For completeness, we verified that our results are not sensitive to the actual energy dependence of the density of states. The continuum states span a finite energy interval centered at the Auger energy $\epsilon_A^{v_1 v_2} = \epsilon_{v_1 v_2} - \epsilon_c$ ($\epsilon_A^{v_1 v_3} = \epsilon_{v_1 v_3} - \epsilon_c$) for region $\mathcal{S}$ ($\mathcal{P}$), where $\epsilon_{v_i v_j}$ is the binding energy of the valence states. Finally, bound and continuum states interact via

$$\begin{aligned} H_{int} = \sum_{k\in\mathcal{S}} U_{kc12} c^\dagger_k c^\dagger_c c_{v_1} c_{v_2} + h.c \\ + \sum_{k\in\mathcal{P}} U_{kc13} c^\dagger_k c^\dagger_c c_{v_1} c_{v_3} + h.c, \end{aligned} \tag{4}$$

where, for simplicity, all interactions with Coulomb integrals with two or more indexes in the continuum are neglected.

The atomic system is excited by an external field described by the atom-light interaction term $H_{ext}(t)$. We choose the laser frequency $\omega$ to be in resonance with the transition $|v_1 v_2\rangle \leftrightarrow |v_1 v_3\rangle$, and assume that $\hbar\omega$ is smaller than the system's ionization potential. Thus,

$$H_{ext}(t) = \Omega f(t) \sin(\omega t) \left( c^\dagger_{v_3} c_{v_2} + c^\dagger_{v_2} c_{v_3} \right), \tag{5}$$

where $f(t)$ is an envelope function due to which the field starts to be applied only at time $t > 0$, $\Omega = \mathcal{E} d$ is the Rabi frequency of the transition, $d = \langle v_2 | x | v_3 \rangle$ the dipole transition element, and $\mathcal{E}$ the field strength of the laser.

As said above, we choose the initial state at time $t = 0$ to have two electrons in the state $|\Psi_0\rangle = |v_1 v_2\rangle$. This, together with the form of the interactions, allows the interacting problem to be reformulated as a non-interacting problem. For this purpose we consider the basis $\mathcal{B} = \{|v_1 v_2\rangle, |v_1 v_3\rangle, |\epsilon_k c\rangle\}$ of two-particle states, where both $H_a$ and $H_c$ are diagonal and have the non-zero matrix elements

$$\langle v_1 v_2 | H_a | v_1 v_2 \rangle = \epsilon_{v_1} + \epsilon_{v_2} + U_{12} \tag{6a}$$

$$\langle v_1 v_3 | H_a | v_1 v_3 \rangle = \epsilon_{v_1} + \epsilon_{v_2} + U_{13} \tag{6b}$$

$$\langle \epsilon_k c | H_c | \epsilon_k c \rangle = \epsilon_k + \epsilon_c. \tag{6c}$$

The interaction Hamiltonian $H_{int}$ only couples states $|v_i v_j\rangle$ to $|\epsilon_k c\rangle$, while $H_{ext}$ only couples states within the

set $\{|v_i v_j\rangle\}$, so that their non-zero matrix elements are given by

$$\langle \epsilon_k c|H_{int}|v_1 v_2\rangle = U_{kc12} \quad (k \in \mathcal{S}) \tag{7a}$$
$$\langle \epsilon_k c|H_{int}|v_1 v_3\rangle = U_{kc13} \quad (k \in \mathcal{P}) \tag{7b}$$
$$\langle v_1 v_3|H_{ext}|v_1 v_2\rangle = \Omega f(t)\sin(\omega t). \tag{7c}$$

The set $\mathcal{B}$ thus constitutes a complete basis for the dynamics. If we define the states $|1\rangle = |v_1 v_2\rangle$, $|2\rangle = |v_1 v_3\rangle$ and $|k\rangle = |\epsilon_k c\rangle$, the Hamiltonian in the two-particle basis can therefore be written as

$$\begin{aligned} H(t) = {}& E_1|1\rangle\langle 1| + E_2|2\rangle\langle 2| + \sum_{k\in\mathcal{S}} E_k|k\rangle\langle k| + \sum_{k\in\mathcal{P}} E_k|k\rangle\langle k| \\ &+ \sum_{k\in\mathcal{S}} M_k(|k\rangle\langle 1| + h.c.) + \sum_{k\in\mathcal{P}} M_k(|k\rangle\langle 2| + h.c.) \\ &+ \Omega f(t)\sin(\omega t)(|2\rangle\langle 1| + |1\rangle\langle 2|), \end{aligned} \tag{8}$$

where $E_1 = \epsilon_{v_1} + \epsilon_{v_2} + U_{12}$, $E_2 = \epsilon_{v_1} + \epsilon_{v_3} + U_{13}$ and $E_k = \epsilon_c + \epsilon_k$. The hopping matrix elements are given by $M_k = U_{kc12}$ for $k \in \mathcal{S}$ and $M_k = U_{kc13}$ for $k \in \mathcal{P}$. Since this Hamiltonian exactly describes the dynamics of the system starting from the state $|\Psi_0\rangle = |v_1 v_2\rangle = |1\rangle$, we use it for the discussion in the main text.

## II. EFFECTIVE EQUATIONS FOR THE ATOMIC SYSTEM

From the discussion above it follows that we can expand the state vector at time $t$ in the basis $\mathcal{B}$ according to

$$\begin{aligned} |\psi(t)\rangle = {}& c_1 e^{-iE_1 t}|1\rangle + c_2 e^{-iE_2 t}|2\rangle \\ &+ \sum_{k\in\mathcal{S}} c_k e^{-iE_k t}|k\rangle + \sum_{k\in\mathcal{P}} c_k e^{-iE_k t}|k\rangle. \end{aligned} \tag{9}$$

This allows us to solve exactly for the coefficients $c_1$ and $c_2$, which are given by

$$\begin{aligned} (i\partial_t - E_1)c_1(t) = {}& \sum_{k\in\mathcal{S}} \int dt' g_k(t-t')|M_k|^2 c_1(t') \\ &+ \Omega f(t)\sin(\omega t)c_2(t), \end{aligned} \tag{10a}$$
$$\begin{aligned} (i\partial_t - E_2)c_2(t) = {}& \sum_{k\in\mathcal{P}} \int dt' g_k(t-t')|M_k|^2 c_2(t') \\ &+ \Omega f(t)\sin(\omega t)c_1(t). \end{aligned} \tag{10b}$$

Here the integral kernel is the non-interacting retarded Green's function $g_k(t-t') = e^{-iE_k(t-t')}\theta(t-t')$. Solving these equations gives the same information about the dynamics of the valence levels $|v_1\rangle$, $|v_2\rangle$ and $|v_3\rangle$ as solving the original Schrödinger equation. However, since we were also interested in the occupations of the continuum states, we found it better to solve the Schrödinger equation directly. We note that these equations can be further simplified by introducing the so-called embedding self-energies

$$\Sigma_{\mathcal{S}}(t-t') = \sum_{k\in\mathcal{S}} g_k(t-t')|M_k|^2 \tag{11a}$$
$$\Sigma_{\mathcal{P}}(t-t') = \sum_{k\in\mathcal{P}} g_k(t-t')|M_k|^2. \tag{11b}$$

In terms of the self-energies the equations for $c_1$ and $c_2$ can be written

$$\begin{aligned} (i\partial_t - E_1)c_1(t) = {}& \int dt' \Sigma_{\mathcal{S}}(t-t')c_1(t') \\ &+ \Omega f(t)\sin(\omega t)c_2(t), \end{aligned} \tag{12a}$$
$$\begin{aligned} (i\partial_t - E_2)c_2(t) = {}& \int dt' \Sigma_{\mathcal{P}}(t-t')c_2(t') \\ &+ \Omega f(t)\sin(\omega t)c_1(t). \end{aligned} \tag{12b}$$

For short times, the probability that a system remains in its initial state decays quadratically with time, and can be written as $P(t) = 1 - t^2/\tau_z^2$ (see next Section), where $\tau_z$ is the Zeno time. In terms of the self-energy above, $\tau_z$ is defined as[3,4]

$$\frac{1}{\tau_z^2} = \frac{1}{\pi}\int dE\, \mathrm{Im}\,\Sigma(E), \tag{13}$$

and will be further discussed in the next Section. At this point we also note that two of the key quantities of the main text, the lifetime and spectral lineshape of the decay process, can be elegantly unified using the theory of non-equilibrium Green's functions (where the self-energy appears as a natural quantity). In this framework, the lifetime is connected to the long time behavior of the lesser Green's function $G^<(t,t)$, while the lineshape can be found from the Fourier transform of the retarded Green's function $G^R(t,t')$[3,4]. However, these quantities are merely aspects of the time-ordered Green's function $G(z,z')$, where the complex arguments lie on the so-called Schwinger-Keldysh contour.

## III. ZENO VS. ANTI-ZENO

It is known that driving a system may induce either a quantum Zeno (QZE) or a so-called quantum anti-Zeno effect (QAZE). A priori, it is not obvious which effect should dominate in our proposed measurement protocol. However, what we find is a clear indication of the Zeno effect. In this section we provide this finding with additional support, and briefly address the differences between our QZE protocol and previous works on the topic.

In the traditional approach to the QZE, we should consider $N$ projective measurements performed in the time interval $[0,T]$, where $T = N\Delta t$ and $\Delta t$ is the time between measurements. This is motivated by the fact that at small enough times, the probability for the system to be in its initial state at the beginning of the first measurement is $P(\Delta t) \approx 1-(\Delta t/\tau_z)^2$, where $1/\tau_z^2 = \langle H^2\rangle - \langle H\rangle^2$

defines the Zeno time $\tau_z$, and the expectation value is taken over the initial state. The probability that at time $T$ the system has not yet decay (the survival probability), is then given by $P(T) = P(\Delta t)^N \approx \left[1 - (T/N\tau_z)^2\right]^N$. In the limit $\Delta t \to 0$ and $N \to \infty$, we find $P(T) = e^{-T^2/N\tau_z^2} \to 1$.

There are two possible issues with the above argument: First, the Zeno time $\tau_z$ is taken to be independent of the measurement period $\Delta t$. This issue has been addressed in a famous paper by Kofman and Kurizki[5], where it was argued that when taking this effect into account, the anti-Zeno effect is more ubiquitous than the Zeno effect. The second issue is with instantaneous projective measurements, which on an ultrafast time-scale are unphysical. It is a crucial point of our protocol that we avoid both these issues: the first by a full time-dependent description of the decay, and the second by explicit modeling of the measurement process (by the external field). For completeness we have however checked that including instantaneous projective measurements in (the end of) our measurement cycle has a marginal effect on our numerical results, and hence we neglect them in the main text. Instead we consider the dipole radiation induce by driving the atomic transition as our principal measurement.

We now discuss the transition from the QZE to the QAZE for our model and protocol. By full exact numerical dynamics, we find that decreasing the time between measurements for $\tau_1 < \tau_2$ gives a transition from unperturbed decay to QZE, with no intermediate QAZE. This was done by using a sequence of measurement pulses (as described in the main text) and varying the time separation between the pulses.

However, for $\tau_1 > \tau_2$, we instead find a QAZE. In contrast to projective schemes, where the QZE to QAZE transition is a function of the measurement frequency (and the density of states[5]), we find that with our approach and system the QZE to QAZE depends *only on system parameters*. Intuitively this feature arises from two aspects of our model: The first is the structure of our model, that consists of two bound states coupled to two separate continua, and the second the explicit modeling of the measurement. To see the significance of these points, assume for a moment that the second bound state is stable: We could then transfer an electron from the Auger decaying state to the stable state, keep it there indefinitely, and then transfer it back. This gives an arbitrary extension of the lifetime, but is not a Zeno effect since no measurements are involved.

To make the above argument more quantitative, and to provide further support to our numerical findings, we present in the following an analytical solution of our model in a simplified limit. We focus the discussion on the Zeno regime (i.e. $\tau_1 < \tau_2$), but the anti-Zeno regime is easily obtained by replacing $\tau_1 \leftrightarrow \tau_2$.

The limit we consider to solve Eqs. 12 exactly is specified by the following assumptions: 1) We invoke the rotating wave approximation. 2) We assume the external field is kept continuously on. 3) We neglect the energy dependence of the self-energy and take $\Sigma(E) \approx -i\Gamma/2$. This last assumption is known in quantum transport language as the wide band limit, and is appropriate for a continuum with large bandwidth and a small system-continuum coupling (both of which hold for our system). Taking the Laplace transform and solving the resulting algebraic equations we find

$$c_1(s) = \frac{s + \Gamma_2}{\Omega^2 + (s + \Gamma_1(s + \Gamma_2)} \tag{14a}$$

$$c_2(s) = -i\frac{\Omega}{\Omega^2 + (s + \Gamma_1)(s + \Gamma_2)}, \tag{14b}$$

where the decay rate are related to the lifetimes by $\Gamma_i = 1/\tau_i$. Transforming back to time we find the probability $P(t) = |c_1(t)|^2 + |c_2(t)|^2$ that the system has not decayed at time $t$ to be

$$P(t) = e^{-(\Gamma_1+\Gamma_2)t/2}\left(1 - \frac{\Gamma_1 + \Gamma_2}{2\beta}\sin(\beta t)\right), \tag{15}$$

where $\beta = \sqrt{4\Omega^2 - (\Gamma_1 - \Gamma_2)^2}$ and we have assumed $4\Omega^2 > (\Gamma_1 - \Gamma_2)^2$. This shows the system decays with an effective decay rate $\Gamma = (\Gamma_1 + \Gamma_2)/2$, which gives a Zeno-like effect for $\tau_1 < \tau_2$.

The above reasoning can be extended to give an approximate description of the effect of using $\pi$-pulses instead of continuous radiation. For this purpose we consider the following measurement cycle: 1) We first drive an electron from state $|1\rangle$ to $|2\rangle$ using a pulse of width $t_\pi = \pi/\Omega$. During this stage we assume the system evolves according to Eq. 15. 2) The system is kept in state $|2\rangle$ for a time $t_m$. 3) A second $\pi$-pulse drives the electron back from state $|2\rangle$ to $|1\rangle$, where again the system evolves according to Eq. 15. 4) Finally we wait a time $t_w$ for the next measurement, during which the system decays as $e^{-\Gamma_1 t_w}$. The full cycle takes a time $t = 2t_\pi + t_m + t_w$, and the survival probability after $n$ cycles will be approximately given by

$$P(nt) \approx \Bigg[e^{-(\Gamma_1+\Gamma_2)t_\pi}\left(1 - \frac{\Gamma_1 + \Gamma_2}{2\beta}\sin(\beta t_\pi)\right)^2 \times e^{-\Gamma_2 t_m} e^{-\Gamma_1 t_w}\Bigg]^n. \tag{16}$$

In the limit where $\Omega$ becomes large, $t_\pi \to 0$ and $\beta \to 2\Omega$, so $P(nt) \approx e^{-\Gamma_2 n t_m} e^{-\Gamma_1 n t_w}$. If also the time between measurements is taken to approach zero, $t \approx t_m$ and $P(nt) \approx e^{-\Gamma_2 n t}$. This indicates that for fast driving and short time between measurements, the system decays with the rate of the upper atomic level. As discussed above this give a Zeno effect if $\tau_1 < \tau_2$, that becomes complete if the upper state is stable ($\Gamma_2 = 0$). These results are consistent with the full numerical calculations in the paper. We wish to note however, that the formulas above should only be applied under the specific assumptions and approximations as discussed. In more general situations, one should solve the full systems dynamics as done in the main text.

## IV. LIFETIMES

We here report the Auger and radiative decay rates of the relevant states in atomic Li and hollow $Li^+$ (see Tab. I and II). These numbers where partially taken from literature, and partially calculated using the GRASP[7,8] atomic structure code. The values in the table show that it is possible to a very good degree to neglect radiative processes in both these systems.

| | Auger$^a$ ($s^{-1}$) $1s^2\,{}^1S_0$ | Radiative$^b$ ($s^{-1}$) |
|---|---|---|
| $1s(2s^2\,{}^1S)\,{}^2S^e$ | $0.0562 \cdot 10^{15}$ | – |
| $1s(2s2p\,{}^3P)\,{}^2P^o$ | $0.0057 \cdot 10^{15}$ | $\sim 10^8$ |

TABLE I. Decay rates from the states $1s2s^2$ and $1s2s2p$ in Li, either by Auger decay or radiative decay.
$^a$ Values taken from Ref. [9]. $^b$ Values taken from Refs. [10] and [11].

| | Auger$^a$ | Radiative$^b$ | | |
|---|---|---|---|---|
| | $1s$ | $1s^2\,{}^1S_0$ | $1s2s\,{}^1S_0$ | $1s3s\,{}^1S_0$ |
| $2s^2\,{}^1S_0$ | $0.258 \cdot 10^{15}$ | – | – | – |
| $2s2p\,{}^1P_1$ | $0.100 \cdot 10^{15}$ | $0.453 \cdot 10^8$ | $0.551 \cdot 10^{11}$ | $0.475 \cdot 10^9$ |

TABLE II. Decay rates (in units of $s^{-1}$) from the states $2s^2$ and $2s2p$ in $Li^+$, into various final states of singly and doubly ionized Li.
$^a$ Values taken from Ref. [12]. $^b$ Values computed with the GRASP atomic structure code.

We also estimated the multi-photon ionization (MPI) rates for Li and $Li^+$ with the PPT model[13–16]. We found an intensity range compatible with our requirements for $\hbar\Omega$, and yet a marginal MPI. Accordingly, where QZE and Auger decay should be observable in Li and $Li^+$ for the range of parameters discussed in the main text.

## V. HOLLOW LI$^+$

We here expand on the discussion in the main text for the results of a hollow $Li^+$ ion. To model this system we identified the excited configuration $2s^2\,{}^1S_0$ with the state $|1\rangle$, and the configuration $2s2p\,{}^1P_1$ with the state $|2\rangle$. We then resonantly drive the dipole accessible transition between these states with a field of frequency $\hbar\omega = 4.1$ eV[12]. Without the measuring field present, the Auger decays from the $2s^2$ and $2s2p$ states happen with respective lifetimes of $\tau_1 = 3.3$ fs and $\tau_2 = 9.7$ fs[12] As shown in Fig 1, the Auger decay from the state $2s^2$ in our model happens with a lifetime $\tau_1 \approx 3.3$ fs when there is no measuring field present. With a laser of intensity 21 TW/cm$^2$ and a measurement time $t_m = 0.32$ fs, the system shows Rabi oscillations between levels $|12\rangle$ and $|13\rangle$ and the lifetime is increased to $\tau_1 \approx 4.7$ fs.

We can also analyze the decay in terms of the occupation $\mathcal{A}(\epsilon_k, t)$ of electrons emitted into the continuum, and detect how the Auger spectral peaks arise in time. In this case (Fig. 1, lower panels) we see that without external field the long-time-limit current gives a single peak in the spectrum. Conversely, when the measurement is performed (i.e. at nonzero field), there are two peaks, resulting from the decay of the $2s^2$ and $2s2p$ levels, that each are split by the dynamical Stark effect into two subpeaks separated by $\Delta\epsilon = \Omega$, for a total of four peaks.

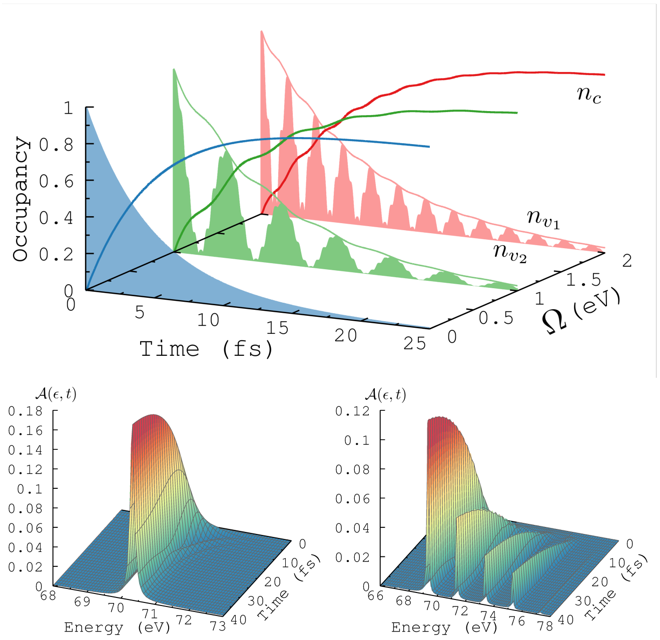


FIG. 1. Auger decay and laser measurement. Top: electron densities $n_c$, $n_{v_1}$ and $n_{v_2}$ of the atomic orbitals as a function of time, for field intensities $I = 0$, 5.3 and 21 TW/cm$^2$ (Rabi frequencies $\Omega = 0$, 1 and 2.1 eV) and measurement time $t_m = 0.32$ fs. The measurement time $t_m = 0.32$ fs. Bottom: Occupation $\mathcal{A}(\epsilon_k, t)$ in the continuum levels $|\epsilon_k\rangle$ as a function of time and energy for $I = 0$ and 21 TW/cm$^2$

## VI. ENTANGLEMENT FORMULAS

For the states $|ij\rangle$ of two spinless particles a convenient entanglement measure is the mode concurrence. This concurrence is defined by[17]

$$\mathcal{C}_{ij} = 2\max\{0, |x| - \sqrt{yz}\}, \quad (17)$$

where $x = \langle c_i^\dagger c_j\rangle$, $y = \langle \hat{n}_i \hat{n}_j\rangle$, and $z = \langle (1-\hat{n}_i)(1-\hat{n}_j)\rangle$. When there is no external field, the only non-zero elements of $\mathcal{C}_{ij}$ are those where $i$ and $j$ correspond to states of the continuum. In our model, each such pair

is initially not entangled, which however changes during the Auger decay due to the terms $U_{kc12}$ and $U_{kc13}$.

## VII. BOUND TO CONTINUUM TRANSITIONS

In the main text we discussed the quantum Zeno effect induced by driving a bound-bound transition. However, the protocol we propose also applies in the case of bound-continuum transitions. To address this point, we consider an atom where the valence levels are less bound, and the state $|v_2\rangle$ is the highest bound state. We assume the field strength $\mathcal{E}$ to be comparable to the Coulomb potential, and the frequency $\hbar\omega$ to be smaller than the ionization potential (IP). In each half-cycle of the laser field, the electron in $|v_2\rangle$ can then tunnel through the Coulomb barrier, accumulate energy in the field, and recombine with the atom in a burst of high-frequency light. This cycle is the mechanism of high harmonic generation (HHG) [18]. The Hamiltonian is as before, but now the atom-laser coupling becomes

$$H_{ext}(t) = \sin(\omega t)\left[\sum_k \Omega_k c_k^\dagger c_{v_2} + \sum_{kk'} \frac{\Omega_{kk'}}{2} c_k^\dagger c_{k'}\right] + h.c., \tag{18}$$

with $\Omega_k = \mathcal{E}\langle v_2|x|k\rangle$ and $\Omega_{kk'} = \mathcal{E}\langle k'|x|k\rangle$ the bound-continuum and continuum-continuum Rabi frequencies, respectively. The interaction of the laser with the deeper levels $|c\rangle$ and $|v_1\rangle$ is omitted, since both tunnel ionization and MPI from these levels should be negligible.

With this laser driving the system will exhibit a QZE, since the HHG signal can be seen as a local measurement probing the presence of a valence electron. During each half-cycle of the field, a fraction $\eta$ of the valence state wave packet is ejected into the continuum. Within one cycle after ejection, this wavepacket fraction returns to the region of the atomic potential to recombine with the remaining wave packet with a probability $P_r$. The probability that an electron is still in level $|v_2\rangle$ after a cycle of duration $t_c$ can therefore be written $P_{v_2}(t_c) = P_{v_2}(0)(1-\eta(1-P_r))$. When the recombination probability becomes close to unity, $P_{v_2}(t_c) \simeq P_{v_2}(0)$ holds to a very good accuracy. However, since the ejected fraction $\eta$ is typically very small ($\eta \sim \mathcal{O}(10^{-4})$), usually $P_{v_2}(t_c) \approx P_{v_2}(0)$ even for the case $P_r < 1$. For $N$ measurements in the interval $[0, T]$ the reasoning is completely analogous to the bound-bound protocol above, with a lower bound on the measurement time given by $t_m > t_c$. Then, for $N \to \infty$, we find the probability $P_{v_2}(T) = \exp\left(-T^2/N\tau_z^2\right)$.

A difference compared to the bound-bound transitions discussed in the main text, is that the quantum Zeno effect now is controlled by tuning the frequency of the external field (as compared to the intensity). This imposes the condition that $\hbar\omega <$ IP in order to not ionize the system. As a proof of principle we have applied the bound-continuum protocol to a model situation with

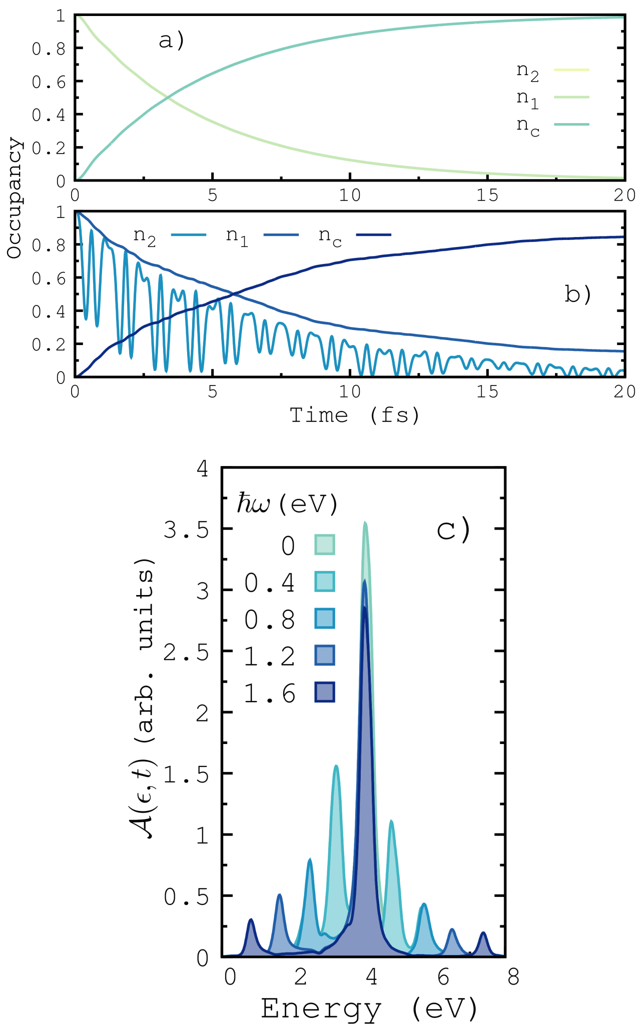


FIG. 2. Bound-to-continuum protocol. Panels a,b): local electron densities $n_c$, $n_1$ and $n_2$ as a function of time, for no field (panel a) and a field of frequency $\hbar\omega = 1.6$ eV and intensity $I = 34$ TW/cm$^2$ (panel b). Panel c) shows the occupation $\mathcal{A}(\epsilon_k, t)$ in the continuum states at $t = 45$ fs, for frequencies $\hbar\omega = 0.0$, 0.4, 0.8, 1.2, 1.6 eV. When increasing $\hbar\omega$, the width of the Auger peak gets reduced.

the same lifetimes as $Li^+$ and an ionization potential IP = 6 eV. Results are shown in Fig. 2a,b. By increasing the frequency $\hbar\omega$ (while maintaining $\hbar\omega <$ IP) the rate of measurements is increased, which leads to an associated increase of the Auger lifetime from 3.3 to 6.3 fs. This change is also visible as a narrowing of the Auger linewidth, shown in Fig. 2c.

## VIII. ESTIMATE OF DIPOLE MATRIX ELEMENTS

To estimate the dipole matrix elements we write the wave function of the continuum state $|k\rangle$ as $\phi_k = e^{ikx}u_k(x)$, where $u_k$ is some envelope function. The po-

sition dependent dipole is then $\Omega_k(x) = E\phi^*_{v_2}(x) x u_k(x)$, with $\phi_{v_2}$ the wave function of state $|v_2\rangle$ centered at $x_0$. If the envelope function is assumed to vary slowly over the width of the function $\phi_{v_2}(x)$, we can take $u_k(x) \simeq u_k(x_0)$, and if the dependence on $k$ can be neglected this further simplifies to

$$\Omega(x) \simeq E\phi^*_{v_2}(x) x u(x_0). \tag{19}$$

In the simple case where the continuum states are approximated as plane waves, and the bound state wave function is described by a Gaussian, we find $\Omega(x) = Exe^{-x^2/\sigma^2}$ and

$$\Omega_k = \int dx \Omega(x) e^{ikx} = -\frac{2iE\sqrt{2}}{\sigma} k e^{-\sigma^2 k^2/4}. \tag{20}$$

Thus both the position and momentum dependent dipole matrix element are in this approximation given by the first derivative of a Gaussian. For the continuum-continuum transitions the same approximations give

$$\Omega(x) \simeq Ex. \tag{21}$$

For the matrix element in momentum space, given by the Fourier transform of the above expression, we find

$$\Omega_{k,k'} \simeq \int dx E x e^{i(k-k')x} = 2\pi i \frac{d}{dq}\delta(q)\big|_{q=k-k'} \tag{22}$$

where the derivative has to be taken in a distributional sense.

---


[1] L. Hedin and S. Lundqvist, Solid State Physics **23**, edited by Seitz et al. (Academic, New York) 1969.

[2] O. Gunnarsson and K. Schönhammer, Phys. Rev. B **22**, 3710 (1980).

[3] Y. Pavlyukh and J. Berakdar, J. Chem. Phys. **135**, 201103 (2011).

[4] Y. Pavlyukh, J. Berakdar, A. and Rubio, Phys. Rev. B **87**, 125101 (2013).

[5] A. G. Kofman and G. Kurizki, Nature **405**, 546 (2000).

[6] A. G. Kofman and G. Kurizki, Phys. Rev. Lett. **93**, 130406 (2004).

[7] C. Froese Fischer, M. Godefroid, T. Brage, P. Jönsson and G.Gaigalas, J. Phys. B: At. Mol. Opt. Phys. **49**,182004 (2016).

[8] P. Jönsson, Gaigalas, J. Bieroń, C. Froese Fischer and I. P. Grant, Comput. Phys. Commun. **184**, 2197 (2013).

[9] G. Verbockhaven and J. E. Hansen, J. Phys. B: At. Mol. Opt. Phys. **34**, 2337 (2001).

[10] M.-K. Chen and K. T. Chung, Phys. Rev. A **49**, 1675 (1994).

[11] J. D. Garcia and J. E. Mack, Phys. Rev. **138**, A987 (1965).

[12] S. Diehl, D. Cubaynes, J.-M. Bizau, F. J. Wuilleumier, E. T. Kennedy, J.-P. Mosnier and T. J. Morgan, J. Phys. B **32**, 4193 (1999)

[13] L. V. Keldysh, Sov.Phys. JETP **20**,1307 (1965).

[14] V. S. Popov, A. M. Perelomov and M. V. Teren'tev, Sov.Phys. JETP **23**, 924 (1966); *ibid.* **24**, 924 (1967) ; **25**, 336 (1967); **26**,222 (1968).

[15] F.A. Ilkov, J.E. Decker and S.L. Chin, J. Phys. B: At. Mol. Opt. Phys. **26**, 4005 (1992).

[16] S.V. Popruzhenko, V. D. Mur, V. S. Popov, and D. Bauer, Phys. Rev. Lett **101**, 193003 (2008).

[17] P. Zanardi and X. Wang, J. Phys. A **35**, 7947 (2002).

[18] see e.g. M. Lewenstein, P. Balcou, M. Y. Ivanov, A. L'Huillier, and P. B. Corkum, Phys. Rev. A **49**, 2117 (1994).
